# Supplementary material for: Adaptive and Explainable Deployment of Navigation Skills via Hierarchical Deep Reinforcement Learning
Source: arXiv:2305.19746 source file (2023-10-30)
Supplement: Supplementary file 1 [file 0_appendix.tex]

\section*{APPENDIX}

Appendixes should appear before the acknowledgment.
